# Supplementary material for: Blueprint First, Model Second: A Framework for Deterministic LLM Workflow
Source: arXiv:2508.02721 source file (2026-06-16)
Supplement: Supplementary file 1 [file appendix.tex]

\section{A Appendix}
\label{sec:appendix}

\subsection{MR6: SemanticNegation}
Since the transformation under MR6 is not semantic-preservation, we define the semantic relations on each task here to ensure the soundness of MR6. Given a source case $\mathcal{X}$, a generated follow-up case $\mathcal{X}^{\prime}$, and a target model $\mathcal{LM}$. 
\begin{itemize}
    \item In MNLI, if the output of $\mathcal{X}$ is "neutral", then $\mathcal{LM}(\mathcal{X}^{\prime})=\mathcal{LM}(\mathcal{X})$, otherwise $\mathcal{LM}(\mathcal{X}^{\prime}) \neq \mathcal{LM}(\mathcal{X})$.
    \item In QQP,  $\mathcal{LM}(\mathcal{X}^{\prime})=\mathcal{LM}(\mathcal{X})$;
    \item In SQuAD2, if the output of $\mathcal{X}$ is "unanswerable", then the output of $\mathcal{X}^{\prime}$ is "unswerable", otherwise $\mathcal{LM}(\mathcal{X}^{\prime}) \neq \mathcal{LM}(\mathcal{X})$.
    \item In NarrativeQA, $Sim(\mathcal{LM(X)}, \mathcal{LM(X)^{\prime}}) < 0.76$.
\end{itemize}

\begin{table}[H]
% \renewcommand{\arraystretch}{1.2}
% \centering
\resizebox{\columnwidth}{!}{
\begin{tabular}{lll}
\hline
Dataset     & Format                          & Train/Test \\ \hline
MNLI        & Etailment/Neutral/Contradiction & 392,702/19,647   \\ \hline
QQP         & Equivalent/Not\_equivalent      & 363,870/40,431   \\ \hline
SQuAD2     & Extractive                      & 130,319/11,873   \\ \hline
NarrativeQA & Abstractive                     & 32,747/3,461    \\ \hline
\end{tabular}}
\caption{The format and statistics of the testing datasets}
\label{tab4}
\end{table}

\subsection{Downstream Tasks and Datasets}

The details about our datasets are shown as follows:

\begin{itemize}
    \item \textbf{MNLI} dataset is a large-scale dataset composed of sentence pairs with textual entailment annotations, where each sentence pair contains a \textit{Premise} and a \textit{Hypothesis}. It is designed to evaluate a model's ability to understand and infer the relationship between the \textit{Premise} and \textit{Hypothesis}. Based on MNLI, NLI is a three-category task, containing three labels: ``entailment'', ``neutral'' and ``contradiction''.
    \item \textbf{QQP} dataset is a collection of question pairs from the community question-answering website Quora, annotated with whether the pairs are semantically equivalent. Based on QQP, DSD is a binary classification task, with labels of ``equivalent'' and ``not\_equivalent''. 
    \item \textbf{SQuAD2} is an extractive reading comprehension dataset in which the contexts, questions, and answers are collected from Wikipedia articles by crowdworkers. Each question's answer in the dataset is a segment or a certain span from the context. SQuAD2 also includes over 50,000 adversarially unanswerable questions, with corresponding answers marked as ``unanswerable''.
    \item \textbf{NarrativeQA} is an abstractive reading comprehension dataset that consists of stories in the form of books and movie scripts. It contains questions that require deep understanding and reasoning over the entire narrative to answer correctly. The answer to each question is not limited to specific spans of text within the story.

\end{itemize}

Table~\ref{tab4} shows the statistics of these four datasets. In particular, the testing set in MNLI contains the matched and mismatched testing sets.

\subsection{Target Models}
In this work, we aim to attack the generative encoder-decoder and decoder-only LLMs and consider BART, LLaMA, and Vicuna as the target LLMs. Specifically, we chose BART-large, the latest development Meta-LLaMA-3-8B, and the version of Vicuna-13b-1.5-16k, where Vicuna-13b-1.5-16k is fine-tuned on LLaMA 2. We select these three LLMs for the following reasons: (1) the target LLMs should be open-source since we need to extract the hidden outputs from them; (2) the target LLMs should be scalable and deployable within our limited computational resources; (3) the target LLMs should achieve state-of-the-art performances on general NLP tasks. As far as we know, these LLMs satisfy the above three requirements and the latter two LLMs achieve over 90\% capability of Bard/ChatGPT~\cite{chiang2023vicuna}. Hence, we consider them the best-fit subject LLMs to deliver representative results and insights. To facilitate the evaluation of model performance, we refer to PromptBench~\cite{zhu2023promptbench} and adopt different task instructions for tasks to guide the model in generating content in a fixed format (shown in Table~\ref{tab5}). In our experiments, all the target models are fine-tuned with LoRa~\cite{hu2021lora}. Through an empirical study, we fine-tune the target models with different sizes of datasets and find that: (i) BART-large achieves the best performances with 1500 cases, and (ii) Vicuna-13B and LLaMA-3-8B achieve the best performances with 600 cases. Table ~\ref{tab6} depicts the accuracy of the fine-tuned target models. Note that the accuracy of each fine-tuned BART-large model on NarrativeQA dataset is less than 35\%, and we do no conduct any experiment in this scenario.

\begin{table}[t]

\centering
\resizebox{0.47\textwidth}{!}{
\begin{tabular}{ccccc}
\hline
Model              & MNLI    & QQP     & SQuAD2  & NqrrativeQA \\ \hline
Vicuna-13B & 85.41\% & 84.90\% & 81.60\% & 80.60\%     \\ \hline
LLaMA-3-8B    & 83.87\% & 83.10\% & 78.70\% & 81.40\%     \\ \hline
BART-large    & 82.06\% & 82.50\% & 76.60\% & --     \\ \hline
\end{tabular}}
\caption{Performances of fine-tuned target LLMs}
\label{tab6}
\end{table}

\begin{table}[t]

\centering
\resizebox{0.48\textwidth}{!}{
\begin{tabular}{ll}
\hline
Task & Task instruction  \\ \hline
NLI  & \begin{tabular}[c]{@{}l@{}}Assess the connection between the following sentences\\ and classify it as "entailment", "neutral", or "contradict- \\ ion": \end{tabular}               \\ \hline
DSD  & \begin{tabular}[c]{@{}l@{}}Can these two statements be considered equal in mean- \\ ing? Answer with "equivalent" or "not\_equivalent": \end{tabular}                             \\ \hline
RC   & \begin{tabular}[c]{@{}l@{}}Discover the best answer of the question based on the\\ context. If the context doesn't include an answer, respo- \\ nd with "unanswerable": \end{tabular} \\ \hline
\end{tabular}}
\caption{Task instructions used to fine-tune target LLMs}
\label{tab5}
\end{table}
